# Supplementary material for: MUX-PLMs: Data Multiplexing for High-throughput Language Models
Source: arXiv:2302.12441 source file (2023-05-22)
Supplement: Supplementary file 1 [file appendix_full_results.tex]

\begin{table*}[t]
    \centering
    % Resize the table
    \resizebox{2\columnwidth}{!}{%
    \begin{tabular}{@{}cclllll@{}}
    
    \toprule
    \multicolumn{1}{l}{\textbf{Architecture}} & \multicolumn{1}{l}{\textbf{Configuration}} & \textbf{Multiplexing} & \textbf{GLUE} & \textbf{NER} & \textbf{POS} & \textbf{Throughput} \\
    \midrule
    \multirow{14}{*}{\textbf{BERT}}           & \multirow{7}{*}{Base}            & None         &      &     &     &            \\
        &                        & \datamux{} (n=2)  &  &  &  &  \\
        &                        & \datamux{} (n=5)  &  &  &  &  \\
        &                        & \datamux{} (n=10) &  &  &  &  \\
        &                        & \pdatamux{} (n=2)  &  &  &  &  \\
        &                        & \pdatamux{} (n=5)  &  &  &  &  \\
        &                        & \pdatamux{} (n=10) &  &  &  &  \\ \cmidrule(lr){2-7}
        & \multirow{7}{*}{Large}  & None &  &  &  &  \\
        &                        & \datamux{} (n=2)  &  &  &  &  \\
        &                        & \datamux{} (n=5)  &  &  &  &  \\
        &                        & \datamux{} (n=10) &  &  &  &  \\
        &                        & \pdatamux{} (n=2)  &  &  &  &  \\
        &                        & \pdatamux{} (n=5)  &  &  &  &  \\
        &                        & \pdatamux{} (n=10) &  &  &  &  \\ \midrule
        \multirow{14}{*}{\textbf{ELECTRA}}           & \multirow{7}{*}{Base}            & None         &      &     &     &            \\
        &                        & \datamux{} (n=2)  &  &  &  &  \\
        &                        & \datamux{} (n=5)  &  &  &  &  \\
        &                        & \datamux{} (n=10) &  &  &  &  \\
        &                        & \pdatamux{} (n=2)  &  &  &  &  \\
        &                        & \pdatamux{} (n=5)  &  &  &  &  \\
        &                        & \pdatamux{} (n=10) &  &  &  &  \\ \cmidrule(lr){2-7}
        & \multirow{7}{*}{Large}  & None &  &  &  &  \\
        &                        & \datamux{} (n=2)  &  &  &  &  \\
        &                        & \datamux{} (n=5)  &  &  &  &  \\
        &                        & \datamux{} (n=10) &  &  &  &  \\
        &                        & \pdatamux{} (n=2)  &  &  &  &  \\
        &                        & \pdatamux{} (n=5)  &  &  &  &  \\
        &                        & \pdatamux{} (n=10) &  &  &  &  \\ 
        \bottomrule
    
    \end{tabular}
    % Resize
    }
    \caption{Full main results}
    \label{app:tab:full_results}
    \end{table*}
